# Supplementary material for: On Scheduler Side-Channels in Dynamic-Priority Real-Time Systems
Source: arXiv:2001.06519 source file (2020-01-17)
Supplement: Supplementary file 1 [file appendix.tex]

% \newpage
\appendix

\section{Appendix Section I}
Appendix
